# Supplementary material for: Transferability in Machine Learning for Electronic Structure via the Molecular Orbital Basis
Source: arXiv:1806.00133 ancillary file (2018-07-26)
Supplement: Supplementary file 1 [file Supporting_Information.pdf]

# Supporting Information for Transferability in Machine Learning for Electronic Structure via the Molecular Orbital Basis

Matthew Welborn, Lixue Cheng, and Thomas F. Miller III
*Division of Chemistry and Chemical Engineering,*
*California Institute of Technology, Pasadena, CA 91125, USA*
(Dated: June 22, 2018)

## I. EXPANDED SMALL MOLECULE PREDICTION STATISTICS

TABLE S1. Detailed decomposition of ML predictions of CCSD correlation energies for the collection of small molecules in Tab. II, with the number of training and testing geometries indicated. Mean and Max Errors are reported for the diagonal ($\Delta\epsilon_{\mathrm{d}}$) and off-diagonal ($\Delta\epsilon_{\mathrm{o}}$) contributions to the correlation energy, as well as the corresponding total and relative correlation energy errors.

| | Geometries | | $\Delta\epsilon_{\mathrm{d}}$(mH) | | $\Delta\epsilon_{\mathrm{o}}$(mH) | | Error (mH) | | Rel. Error(%) | |
|---|---|---|---|---|---|---|---|---|---|---|
| Molecule | Train | Test | Mean | Max | Mean | Max | Mean | Max | Mean | Max |
| $H_2$ | 50 | 100 | 0.002 | 0.005 | NA | NA | 0.00 | 0.00 | 0.00 | 0.01 |
| $N_2$ | 50 | 100 | 0.016 | 0.202 | 0.008 | 0.052 | 0.06 | 0.19 | 0.01 | 0.05 |
| $F_2$ | 50 | 100 | 0.003 | 0.037 | 0.002 | 0.014 | 0.03 | 0.18 | 0.00 | 0.03 |
| HF | 50 | 100 | 0.002 | 0.050 | 0.005 | 0.064 | 0.03 | 0.23 | 0.01 | 0.08 |
| $NH_3$ | 50 | 100 | 0.026 | 0.112 | 0.014 | 0.056 | 0.16 | 0.57 | 0.06 | 0.23 |
| $CH_4$ | 50 | 100 | 0.013 | 0.088 | 0.006 | 0.051 | 0.03 | 0.10 | 0.01 | 0.05 |
| CO | 50 | 100 | 0.002 | 0.009 | 0.027 | 0.073 | 0.03 | 0.07 | 0.01 | 0.02 |
| $CO_2$ | 50 | 100 | 0.005 | 0.027 | 0.004 | 0.087 | 0.04 | 0.17 | 0.01 | 0.03 |
| HCN | 50 | 100 | 0.006 | 0.030 | 0.007 | 0.050 | 0.04 | 0.17 | 0.01 | 0.05 |
| HNC | 50 | 100 | 0.016 | 0.218 | 0.012 | 0.072 | 0.09 | 0.45 | 0.03 | 0.13 |
| $C_2H_2$ | 50 | 100 | 0.032 | 0.193 | 0.023 | 0.137 | 0.21 | 0.61 | 0.06 | 0.19 |
| $C_2H_4$ | 50 | 100 | 0.041 | 0.344 | 0.016 | 0.155 | 0.30 | 0.75 | 0.08 | 0.21 |
| $C_2H_6$$^\dagger$ | 50 | 1000 | 0.037 | 0.460 | 0.014 | 0.101 | 0.33 | 1.27 | 0.08 | 0.31 |
| | 200 | 1000 | 0.028 | 0.413 | 0.011 | 0.108 | 0.21 | 1.22 | 0.05 | 0.30 |
| $CH_2O$ | 50 | 100 | 0.012 | 0.091 | 0.010 | 0.099 | 0.09 | 0.33 | 0.02 | 0.08 |
| $HCO_2H$$^\dagger$ | 50 | 1000 | 0.036 | 0.288 | 0.020 | 0.341 | 0.40 | 1.24 | 0.06 | 0.19 |
| | 100 | 1000 | 0.026 | 0.522 | 0.015 | 0.375 | 0.27 | 0.86 | 0.04 | 0.14 |
| $CH_3OH$ | 50 | 100 | 0.018 | 0.073 | 0.013 | 0.078 | 0.14 | 0.55 | 0.03 | 0.12 |
| $CH_2F_2$$^\dagger$ | 50 | 1000 | 0.044 | 1.709 | 0.023 | 0.691 | 0.73 | 2.94 | 0.11 | 0.43 |
| | 100 | 1000 | 0.035 | 0.724 | 0.018 | 0.560 | 0.56 | 2.05 | 0.08 | 0.30 |
| $C_6H_6$ | 50 | 100 | 0.023 | 0.235 | 0.009 | 0.170 | 0.30 | 1.19 | 0.03 | 0.12 |
| $H_2O$$^\ddagger$ | | | | | | | | | | |
| *cc-pVDZ* | 50 | 200 | 0.017 | 0.097 | 0.008 | 0.063 | 0.05 | 0.22 | 0.02 | 0.10 |
| *cc-pVTZ* | 50 | 200 | 0.014 | 0.077 | 0.010 | 0.050 | 0.04 | 0.14 | 0.02 | 0.05 |
| *cc-pVQZ* | 50 | 200 | 0.015 | 0.081 | 0.011 | 0.057 | 0.05 | 0.20 | 0.02 | 0.07 |
| *cc-pV5Z* | 50 | 200 | 0.018 | 0.109 | 0.012 | 0.055 | 0.08 | 0.37 | 0.03 | 0.13 |

$^\dagger$ Two sizes of training sets are presented to illustrate error reduction. $^\ddagger$ Results for several basis sets provided.

## II. MACHINE LEARNING MP2 PREDICTIONS

TABLE S2. As for Tab. S1, but with MP2 correlation energies rather than CCSD.

| | Geometries | | $\Delta\epsilon_d$(mH) | | $\Delta\epsilon_o$(mH) | | Error(mH) | | Rel. Error(%) | |
|---|---|---|---|---|---|---|---|---|---|---|
| Molecule | Train | Test | Mean | Max | Mean | Max | Mean | Max | Mean | Max |
| $H_2$ | 50 | 100 | 0.003 | 0.005 | NA | NA | 0.00 | 0.00 | 0.01 | 0.02 |
| $N_2$ | 50 | 100 | 0.014 | 0.163 | 0.013 | 0.233 | 0.15 | 0.48 | 0.04 | 0.12 |
| $F_2$ | 50 | 100 | 0.003 | 0.064 | 0.002 | 0.013 | 0.04 | 0.33 | 0.01 | 0.06 |
| HF | 50 | 100 | 0.003 | 0.047 | 0.004 | 0.059 | 0.03 | 0.28 | 0.01 | 0.10 |
| $NH_3$ | 50 | 100 | 0.023 | 0.119 | 0.016 | 0.067 | 0.14 | 0.50 | 0.06 | 0.21 |
| $CH_4$ | 50 | 100 | 0.012 | 0.077 | 0.007 | 0.049 | 0.03 | 0.11 | 0.02 | 0.05 |
| CO | 50 | 100 | 0.004 | 0.015 | 0.005 | 0.023 | 0.03 | 0.10 | 0.01 | 0.03 |
| $CO_2$ | 50 | 100 | 0.005 | 0.029 | 0.004 | 0.083 | 0.03 | 0.17 | 0.00 | 0.03 |
| HCN | 50 | 100 | 0.006 | 0.036 | 0.007 | 0.065 | 0.04 | 0.23 | 0.01 | 0.07 |
| HNC | 50 | 100 | 0.011 | 0.055 | 0.011 | 0.281 | 0.08 | 0.46 | 0.02 | 0.14 |
| $C_2H_2$ | 50 | 100 | 0.025 | 0.145 | 0.022 | 0.219 | 0.24 | 0.80 | 0.08 | 0.26 |
| $C_2H_4$ | 50 | 100 | 0.034 | 0.200 | 0.015 | 0.359 | 0.26 | 0.85 | 0.08 | 0.25 |
| $C_2H_6{}^\dagger$ | 50 | 1000 | 0.035 | 1.286 | 0.013 | 0.129 | 0.36 | 2.28 | 0.10 | 0.61 |
| | 150 | 1000 | 0.022 | 0.416 | 0.010 | 0.102 | 0.17 | 0.97 | 0.05 | 0.26 |
| $CH_2O$ | 50 | 100 | 0.009 | 0.088 | 0.011 | 0.144 | 0.10 | 0.36 | 0.03 | 0.09 |
| $HCO_2H^\dagger$ | 50 | 1000 | 0.031 | 0.281 | 0.020 | 0.357 | 0.36 | 1.67 | 0.06 | 0.26 |
| | 100 | 1000 | 0.025 | 0.240 | 0.015 | 0.182 | 0.28 | 0.96 | 0.04 | 0.15 |
| $CH_3OH$ | 50 | 100 | 0.015 | 0.070 | 0.013 | 0.091 | 0.14 | 0.72 | 0.03 | 0.17 |
| $CH_2F_2{}^\dagger$ | 50 | 1000 | 0.035 | 1.266 | 0.023 | 0.863 | 0.54 | 3.79 | 0.08 | 0.56 |
| | 100 | 1000 | 0.024 | 0.461 | 0.018 | 0.512 | 0.35 | 2.18 | 0.05 | 0.32 |
| $C_6H_6$ | 50 | 100 | 0.021 | 0.151 | 0.009 | 0.197 | 0.34 | 1.20 | 0.04 | 0.13 |
| $H_2O^\ddagger$ | | | | | | | | | | |
| *cc-pVDZ* | 50 | 200 | 0.019 | 0.098 | 0.012 | 0.075 | 0.09 | 0.35 | 0.04 | 0.17 |
| *cc-pVTZ* | 50 | 200 | 0.018 | 0.084 | 0.014 | 0.069 | 0.10 | 0.42 | 0.04 | 0.16 |
| *cc-pVQZ* | 50 | 200 | 0.020 | 0.097 | 0.015 | 0.081 | 0.09 | 0.35 | 0.03 | 0.12 |
| *cc-pV5Z* | 50 | 200 | 0.016 | 0.090 | 0.013 | 0.062 | 0.11 | 0.44 | 0.03 | 0.15 |

† Two sizes of training sets are presented to illustrate error reduction. ‡ Results for several basis sets provided.

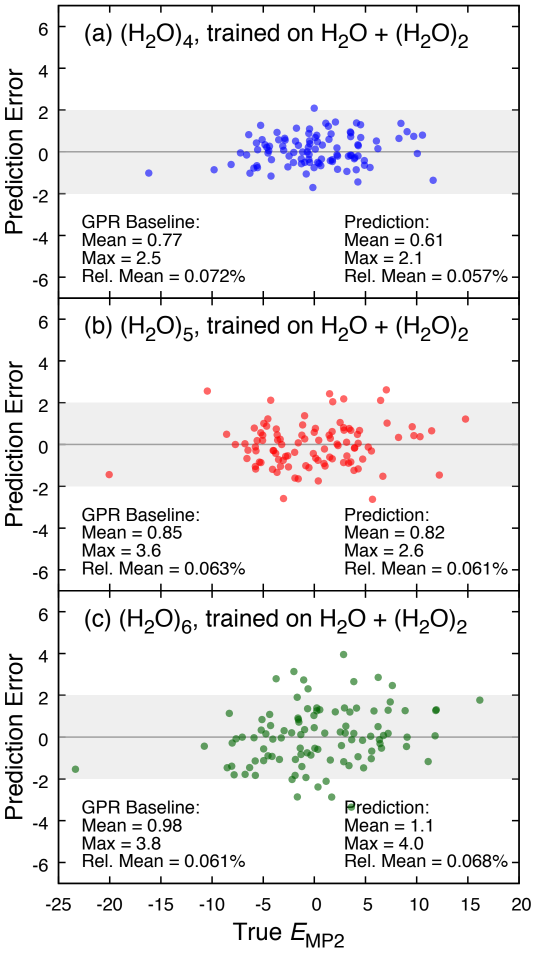


FIG. S1. As for Fig. 2, but with MP2 in place of CCSD. Parallelity error is removed via a global shift in the predicted energies of the tetramer, pentemer, and hexamer by 0.68, 0.40, and 0.38 mH, respectively.

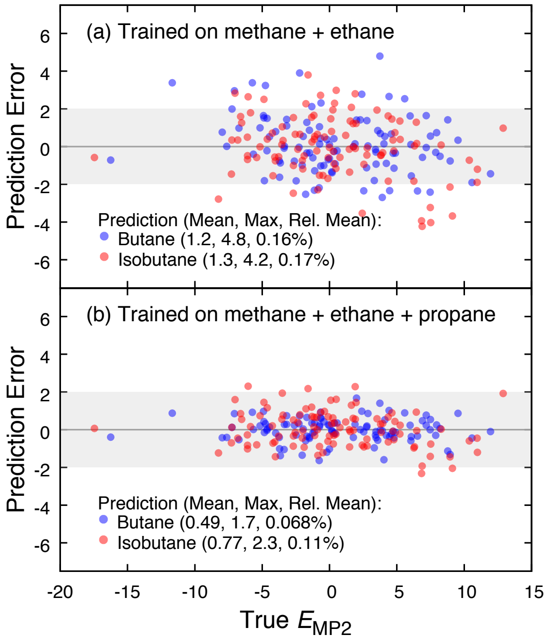


FIG. S2. As for Fig. 3, but with MP2 in place of CCSD. Parallelity error is removed via a global shift in the predicted energies of butane and isobutane by (a) 32 and 21 mH and (b) 3.3 and 0.87 mH, respectively. The Mean and Max GPR baseline errors for butane are 0.40 and 1.2 mH, respectively. For isobutane, these errors are 0.47 and 1.7 mH.

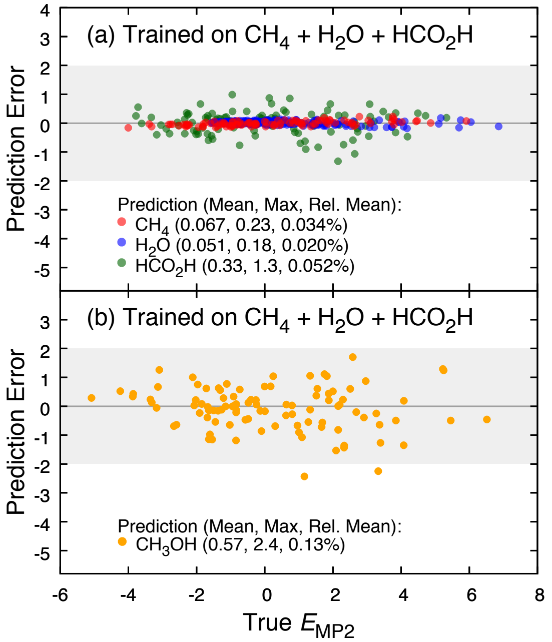


FIG. S3. As for Fig. 4, but with MP2 in place of CCSD. In panel (b), parallelity error is removed via a global shift in the predicted energy by 4.5 mH.

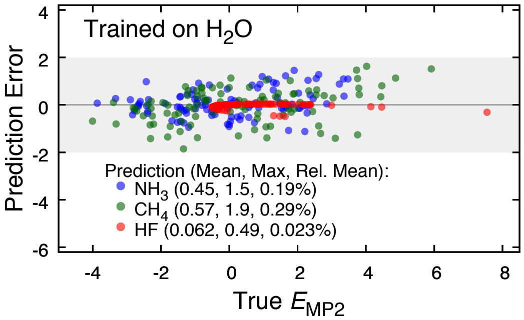


FIG. S4. As for Fig. 5, but with MP2 in place of CCSD. Parallelity error is removed via a global shift in the predicted energies of ammonia, methane, and hydrogen fluoride by 24, 51, and 12 mH, respectively.

## III. MACHINE LEARNING PREDICTION ERRORS PLOTTED IN TERMS OF TOTAL ENERGIES

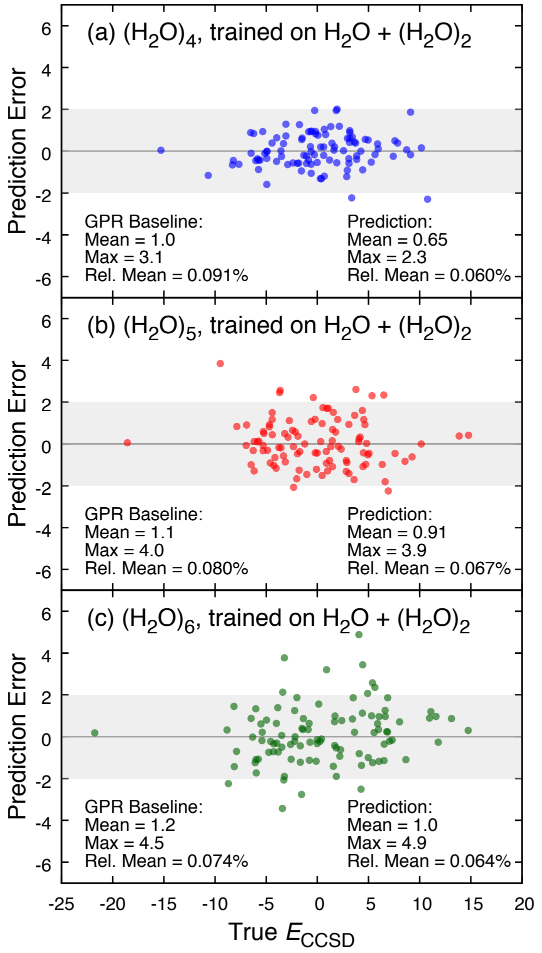


FIG. S5. As for Fig. 2, except plotting ML predictions of CCSD total energies versus true CCSD total energies.

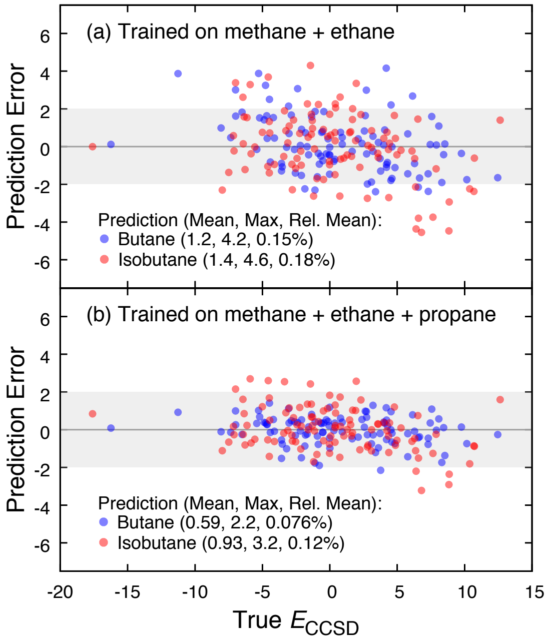


FIG. S6. As for Fig. 3, except plotting ML predictions of CCSD total energies versus true CCSD total energies.

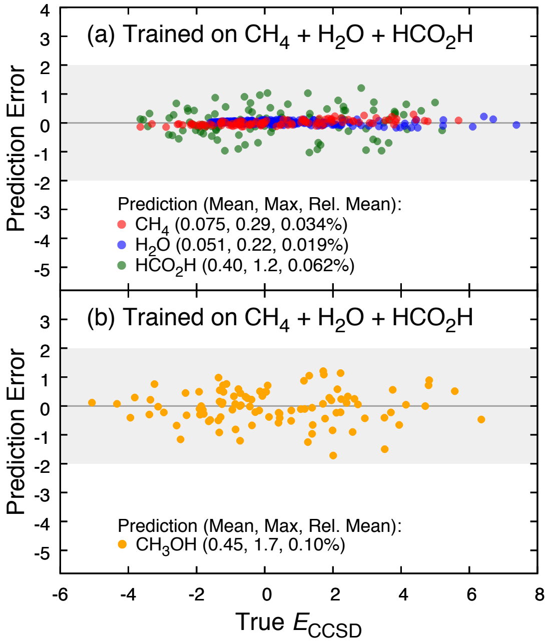


FIG. S7. As for Fig. 4, except plotting ML predictions of CCSD total energies versus true CCSD total energies.

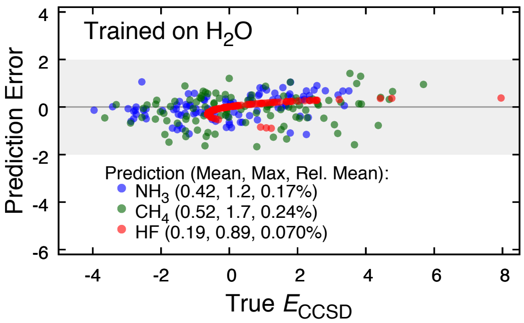


FIG. S8. As for Fig. 5, except plotting ML predictions of CCSD total energies versus true CCSD total energies.
